# Supplementary material for: VIAFormer: Voxel-Image Alignment Transformer for High-Fidelity Voxel Refinement
Source: arXiv:2601.13664 source file (2026-01-21)
Supplement: Supplementary file 1 [file suppl.tex]

\documentclass[10pt,twocolumn,letterpaper]{article}
\usepackage[rebuttal]{cvpr}

% Include other packages here, before hyperref.
\usepackage{graphicx}
\usepackage{amsmath}
\usepackage{amssymb}
\usepackage{booktabs}

% Import additional packages in the preamble file, before hyperref
\input{preamble}

% If you comment hyperref and then uncomment it, you should delete
% egpaper.aux before re-running latex.  (Or just hit 'q' on the first latex
% run, let it finish, and you should be clear).
\definecolor{cvprblue}{rgb}{0.21,0.49,0.74}
\usepackage[pagebackref,breaklinks,colorlinks,allcolors=cvprblue]{hyperref}

% If you wish to avoid re-using figure, table, and equation numbers from
% the main paper, please uncomment the following and change the numbers
% appropriately.
%\setcounter{figure}{2}
%\setcounter{table}{1}
%\setcounter{equation}{2}

% If you wish to avoid re-using reference numbers from the main paper,
% please uncomment the following and change the counter value to the
% number of references you have in the main paper (here, 100).
%\makeatletter
%\apptocmd{\thebibliography}{\global\c@NAT@ctr 100\relax}{}{}
%\makeatother

%%%%%%%%% PAPER ID  - PLEASE UPDATE
 % *** Enter the Paper ID here

\begin{document}

%%%%%%%%% TITLE - PLEASE UPDATE
\title{VIAFormer: Voxel-Image Alignment Transformer for\\ High-Fidelity Voxel Refinement}  % **** Enter the paper title here

\twocolumn[{
\renewcommand\twocolumn[1][]{#1}
\maketitlesupplementary
}]
\appendix

\input{sec/X_suppl_2}

%%%%%%%%% REFERENCES
{
    \small
    \bibliographystyle{ieeenat_fullname}
    \bibliography{main}
}

\end{document}
